# Supplementary material for: Towards Diverse Behaviors: A Benchmark for Imitation Learning with Human Demonstrations
Source: arXiv:2402.14606 source file (2024-02-22)
Supplement: Supplementary file 5 [file appendix.tex]

\section{Other}

%%%%%%%%%%%%%%%%%%%%%%%%%%%%%%%%%%%%%%%%%%%%%%%%%%%%%%%
% \begin{table}[hbtp]
% \centering
%  % \caption{Overview of Tasks.}\label{task_summary}
% \resizebox{0.5\textwidth}{!}{  
% \begin{tabular}{l|ccc}
% 	\toprule 
%          Tasks &  \multicolumn{2}{c}{$\text{dim} (\mathcal{S})$ }  &  $\text{dim} (\mathcal{A})$  \\
%           & state-based & image-based  & \\
% 	\midrule
%         Avoiding  & 4 & - & 2 \\          
%         Pushing &  10 & - & 2 \\
%         Aligning &  20 & $(2, 3, 96, 96)$ & 3 \\
%         Sorting-X & $4 + 6\text{X}$ & $(2, 3, 96, 96)$ & 8 \\
%         Stacking & 20 & $(2, 3, 96, 96)$ & 8 \\  
% 	\bottomrule
% \end{tabular}
% }
% \vskip -0.15in
% \end{table}
%%%%%%%%%%%%%%%%%%%%%%%%%%%%%%%%%%%%%%%%%%%%%%%%%%%%%%%
%  \begin{wrapfigure}{r}{0.4\textwidth}
% \includegraphics[width=.48\linewidth]{figures/tasks2/front_15.jpg} 
% \includegraphics[width=.48\linewidth]{figures/tasks2/inhand_15.jpg} 
% \caption{Camera views. Front view (right) and in-hand (left).}
% \label{fig:wrapfig}
% \end{wrapfigure}

\subsection{Full Results}
This section provides more results what are missed in the main page.
